# Supplementary material for: On the use of Solomon echoes in 27Al NMR studies of complex aluminium hydrides
Source: arXiv:2211.01039 ancillary file (2022-11-02)
Supplement: Supplementary file 1 [file SolomonSupp.pdf]

Supporting Information:  
On the use of Solomon echoes in  $^{27}\text{Al}$  NMR studies of  
complex aluminium hydrides

Michael Fischer and Bodo Zibrowius

Table S1: Results of GIPAW-DFT calculations (The convention  $\sigma_{11} \leq \sigma_{22} \leq \sigma_{33}$  is used to assure that the span  $\Omega = \sigma_{33} - \sigma_{11}$  is positive.)

| Material                              | Space group    | $C_Q/\text{MHz}$ | $\eta$ | $\sigma_{11}/\text{ppm}$ | $\sigma_{22}/\text{ppm}$ | $\sigma_{33}/\text{ppm}$ | $\sigma_{iso}/\text{ppm}$ |
|---------------------------------------|----------------|------------------|--------|--------------------------|--------------------------|--------------------------|---------------------------|
| $\text{LiAlH}_4$                      | $P2_1/c^1$     | 3.618            | 0.33   | 446.17                   | 451.75                   | 466.43                   | 454.78                    |
| $\text{Li}_3\text{AlH}_6(\text{Al1})$ | $R\bar{3}^2$   | 2.538            | 0      | 598.66                   | 598.66                   | 603.12                   | 600.15                    |
| $\text{Li}_3\text{AlH}_6(\text{Al2})$ |                | -1.540           | 0      | 594.62                   | 606.69                   | 606.69                   | 602.67                    |
| $\text{Na}_3\text{AlH}_6$             | $P2_1/n^3$     | -1.019           | 0.50   | 600.52                   | 610.48                   | 611.63                   | 607.54                    |
| $\text{Na}_2\text{LiAlH}_6$           | $Fm\bar{3}m^4$ | 0                | 0      | 625.99                   | 625.99                   | 625.99                   | 625.99                    |
| $\text{KAlH}_4$                       | $Pnma^5$       | -1.693           | 0.59   | 446.32                   | 447.34                   | 451.63                   | 448.43                    |
| $\text{NaAlH}_4$                      | $I4_1/a^6$     | 3.139            | 0      | 454.98                   | 454.98                   | 474.23                   | 461.39                    |
| $\text{NaAlH}_4$                      | $I4_1/a^3$     | 3.142            | 0      | 454.88                   | 454.88                   | 474.20                   | 461.32                    |

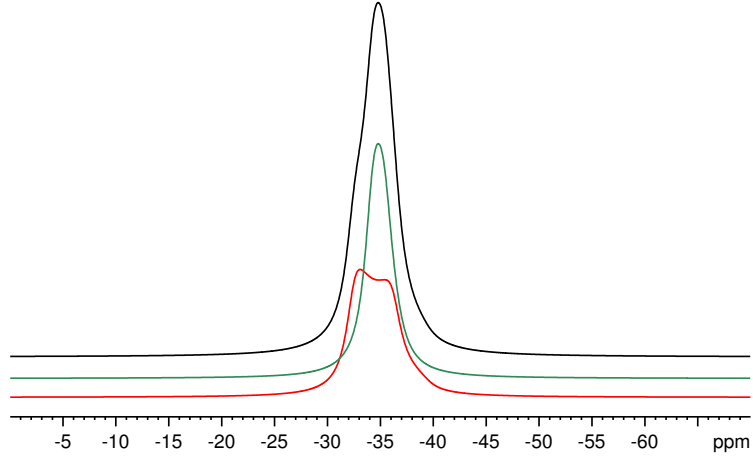

Figure S1: Simulated  $^{27}\text{Al}$  MAS NMR spectrum of  $\text{Li}_3\text{AlH}_6$  at a resonance frequency of 104 MHz. For the simulation the following parameters were used:  $\delta_{iso} = -31.2/-33.7$  ppm and  $|C_Q| = 2.54/1.54$  MHz for Al1 (red) and Al2 (green), respectively. For both lines, a Lorentzian line broadening  $LB = 200$  Hz was used. Based on these parameters, the resulting resonance line (black) is only slightly asymmetric and has a width (FWHM) of only about 400 Hz corresponding to less than 3.9 ppm.

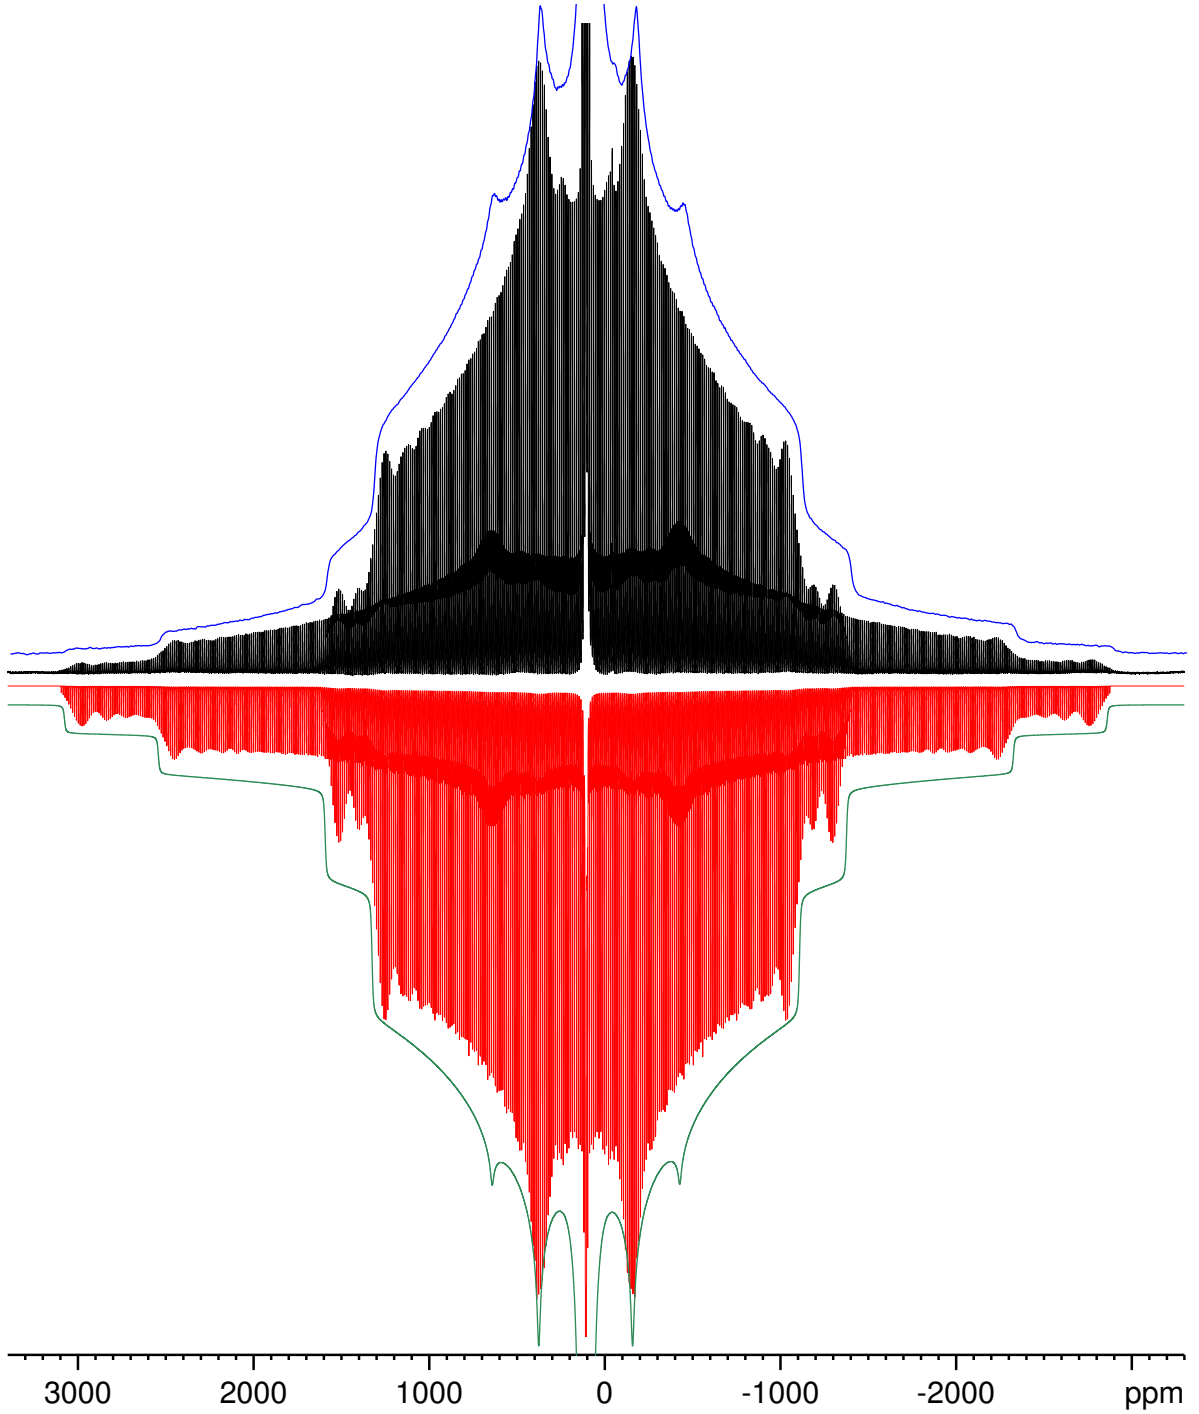

Figure S2: Experimental  $^{27}\text{Al}$  NMR spectra of measured for a stationary sample (blue) and the same sample spinning at  $\nu_{MAS} = 1.4$  kHz (black) and their simulations (green and red, respectively) with the parameters  $\delta_{iso} = 107.6$  ppm,  $C_Q = 1.29$  MHz and  $\eta = 0.64$ . To ease the comparison, the simulated spectra have been inverted.

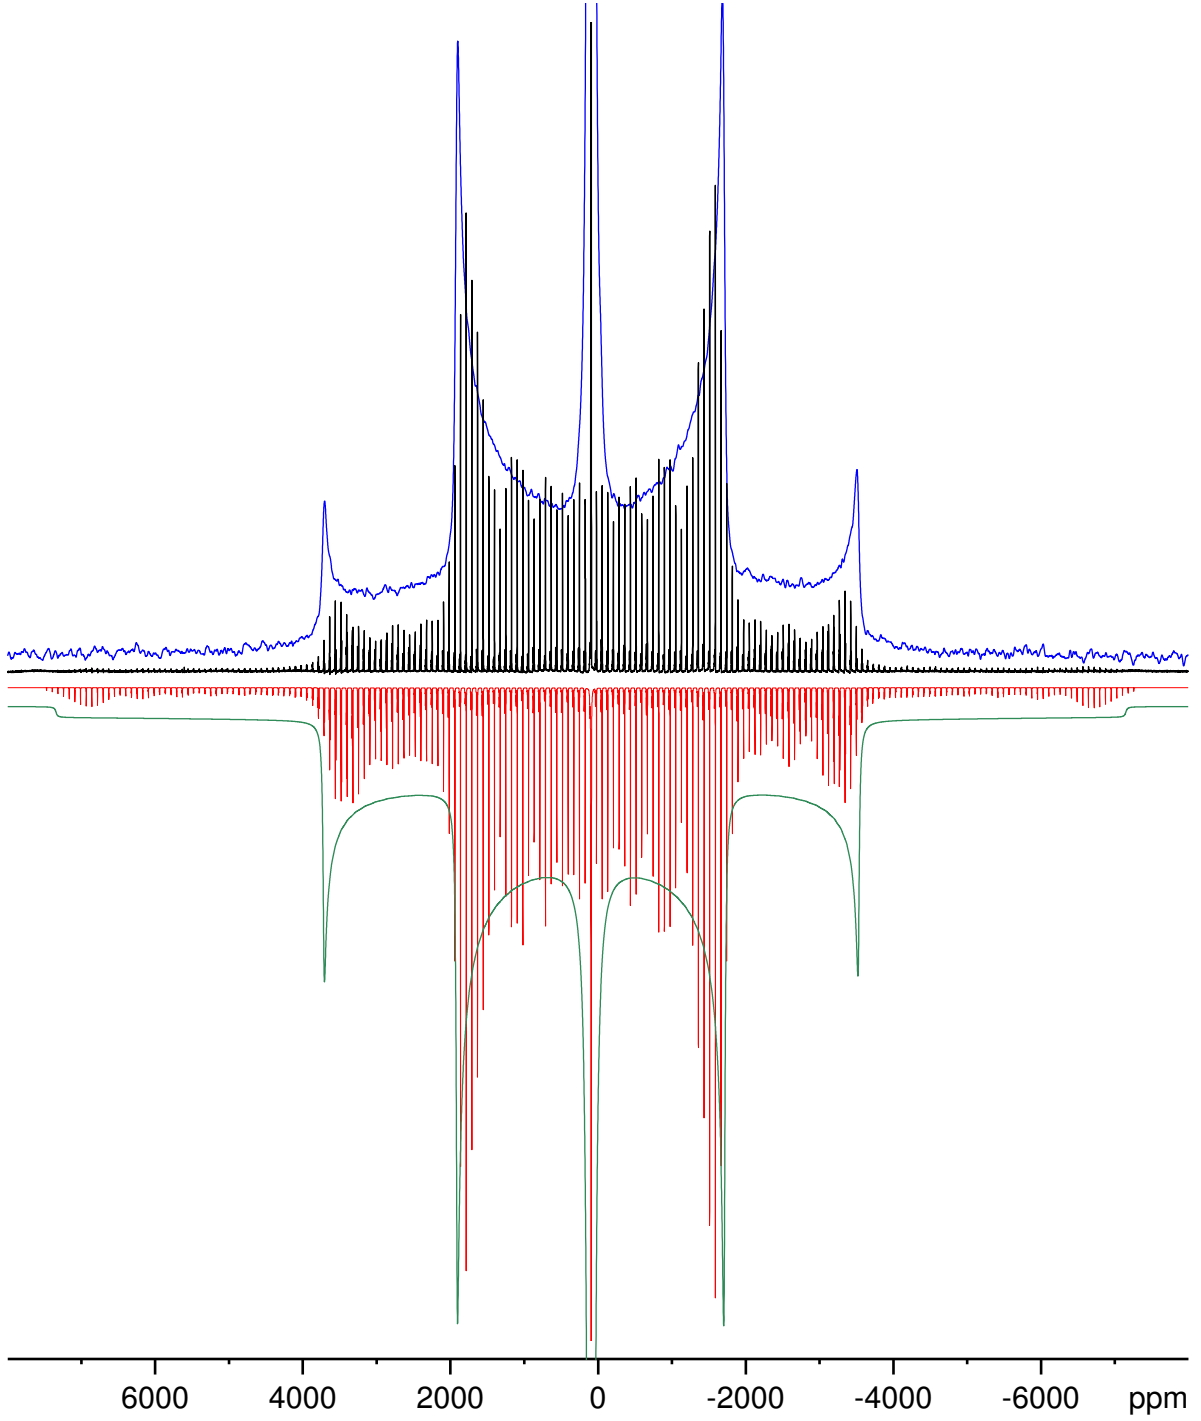

Figure S3: Experimental  $^{27}\text{Al}$  NMR spectra of  $\text{NaAlH}_4$  measured for a stationary sample (blue) and the same sample spinning at  $\nu_{MAS} = 10$  kHz (black) and their simulations (green and red, respectively) with the parameters  $\delta_{iso} = 97.2$  ppm,  $C_Q = 3.11$  MHz and  $\eta = 0$ . To ease the comparison, the simulated spectra have been inverted.

## References

- (1) Hauback, B. C.; Brinks, H. W.; Fjellvåg, F. *J. Alloys Compd.* **2002**, *346*, 184–189.
- (2) Brinks, H. W.; Hauback, B. C. *J. Alloys Compd.* **2003**, *354*, 143–147.
- (3) Ozolins, V.; Majzoub, E.; Udovic, T. *J. Alloys Compd.* **2004**, *375*, 1–10.
- (4) Brinks, H. W.; Hauback, B. C.; Jensen, C. M.; Zidan, R. *J. Alloys Compd.* **2005**, *392*, 27–30.
- (5) Zibrowius, B.; Felderhoff, M. *Phys. Chem. Chem. Phys.* **2019**, *21*, 12576–12584.
- (6) Hauback, B. C.; Brinks, H. W.; Jensen, C. M.; Murphy, K.; Maeland, A. J. *J. Alloys Compd.* **2003**, *358*, 142–145.
